# Supplementary material for: Energy-Efficient Ultrashort-Pulse Characterization using Nanophotonic Parametric Amplification
Source: arXiv:2501.11152 source file (2025-01-19)
Supplement: Supplementary file 1 [file Supplemental.tex]

\section{Detailed workflow}
Figure \ref{fig:sup-workflow} (a) shows the detailed experimental setup used for DOPA-XFROG. 
A $100fs$ mode-locked fiber laser centered at $1045nm$ is used to pump a home-built optical parametric oscillator (OPO) and as the gate for the DOPA-XFROG. 
The output of the OPO is at $2090nm$ which is used as the "Unknown pulse" to be characterized. 
Both the pump and OPO output are characterized with a traditional table-top XFROG to create the reference pulses seen in Fig. \ref{fig:Results} (Right). 
The output of the OPO is gated by the pump in the nanophotonic OPA for different delays controlled by a linearized motor stage. 
The resulting signal from the OPA is low-pass filtered and collected in a spectrometer and slow detector. 
The stage is set to scan continuously and the spectrometer measures the spectrum as a function of delay one wavelength component at a time from $1790 nm$ to $2390 nm$ with a bandwidth of $2nm$.   
The analog output of the spectrometer is amplified using a voltage preamplifier and sent to an oscilloscope. 
The signal collected by the slow detector used for calibration during postprocessing is also sent to the same oscilloscope. 
The oscilloscope is set to trigger data collection when the slow detector signal passes a threshold voltage level indicating temporal overlap of the two pulses for each scan of the delay stage.
Between subsequent scans, the spectrometer updates the collected wavelength center by $2nm$. 
The detector and spectrometer traces are saved on the oscilloscope for each stage scan to create the calibration matrix and raw spectrogram in Fig. \ref{fig:sup-workflow} (b, Left). 
The calibration matrix and raw spectrogram are then passed through the postprocessing algorithm described in Section \ref{sec:sup-postproc} which produces a calibrated spectrogram (Fig. \ref{fig:sup-workflow} (b, Right)). 
The calibrated spectrogram can now be used with the DOPA-XFROG recovery algorithm to recover the intensity and phase of the unknown pulse (See Fig. \ref{fig:sup-workflow} (c)). 

\begin{figure*}[b] % left,bottom,right,top
	\begin{centering}
    	 %\fbox{
    	% \makebox[\textwidth][c]{
    		\includegraphics[width=1\linewidth,trim={0cm 2cm 0cm 4cm},clip]{Figures/DetailedWorkflow3.pdf}
    	% }
    	 % }
    	\par\end{centering}
        \caption{ \textbf{Workflow.} \textbf{(a)} Detailed experimental setup. BS: Beam Splitter; OPO: Optical Parametric Oscillator; DM: Dichroic Mirror; OPA: Optical Parametric Amplifier; LPF: Low Pass Filter; DET: Detector. \textbf{b} The calibration matrix, consisting of the measured detector signal, calibrates the spectrogram in postprocessing. 
        \textbf{(c)} The processed spectrogram is passed through the recovery algorithm for pulse retrieval.  
    	}
	\label{fig:sup-workflow}
\end{figure*}

\begin{comment}
\section{Device design and fabrication}
The design and fabrication of the dispersion-engineered nanophotonic OPA used here follow the techniques described by Ledezma et al \cite{ledezma2022intense}.
The waveguides were designed to have minimal dispersion and walk-off between the signal at $2090 nm$ and pump at $1045nm$.   
The waveguides were etched on a 704nm thin film of lithium niobate on a silica substrate and were measured using atomic force microscopy to have a top width of 1790nm and an etch depth of 330nm. 
The etched waveguide geometry was simulated using Lumerical to estimate a group velocity mismatch between $1045nm$ and $2090nm$ of $1.7fs/mm$, group velocity dispersion around $2090 nm$ of $-3 fs^2 /mm$, group velocity dispersion around $1045 nm$ of $54 fs^2 /mm$. 
The total length of the waveguide was $10mm$ with a periodically poled region $4mm$ long with a poling period of $5.2um$. 
The OPA was measured (using the technique described in \cite{ledezma2022intense}) to have a gain of 188dB/cm and a bandwidth of 40.5THz marking, to our knowledge, the highest integrated gain-bandwidth of any optical amplifier recorded to date.  
\end{comment}

\section{Postprocessing}
\label{sec:sup-postproc}
\begin{figure}[b] % left,bottom,right,top
	\begin{centering}
    	% \fbox{
    % 	\makebox[\textwidth][c]{
    		\includegraphics[width=1\linewidth,trim={1.5cm 3.3cm 3cm 1cm},clip]{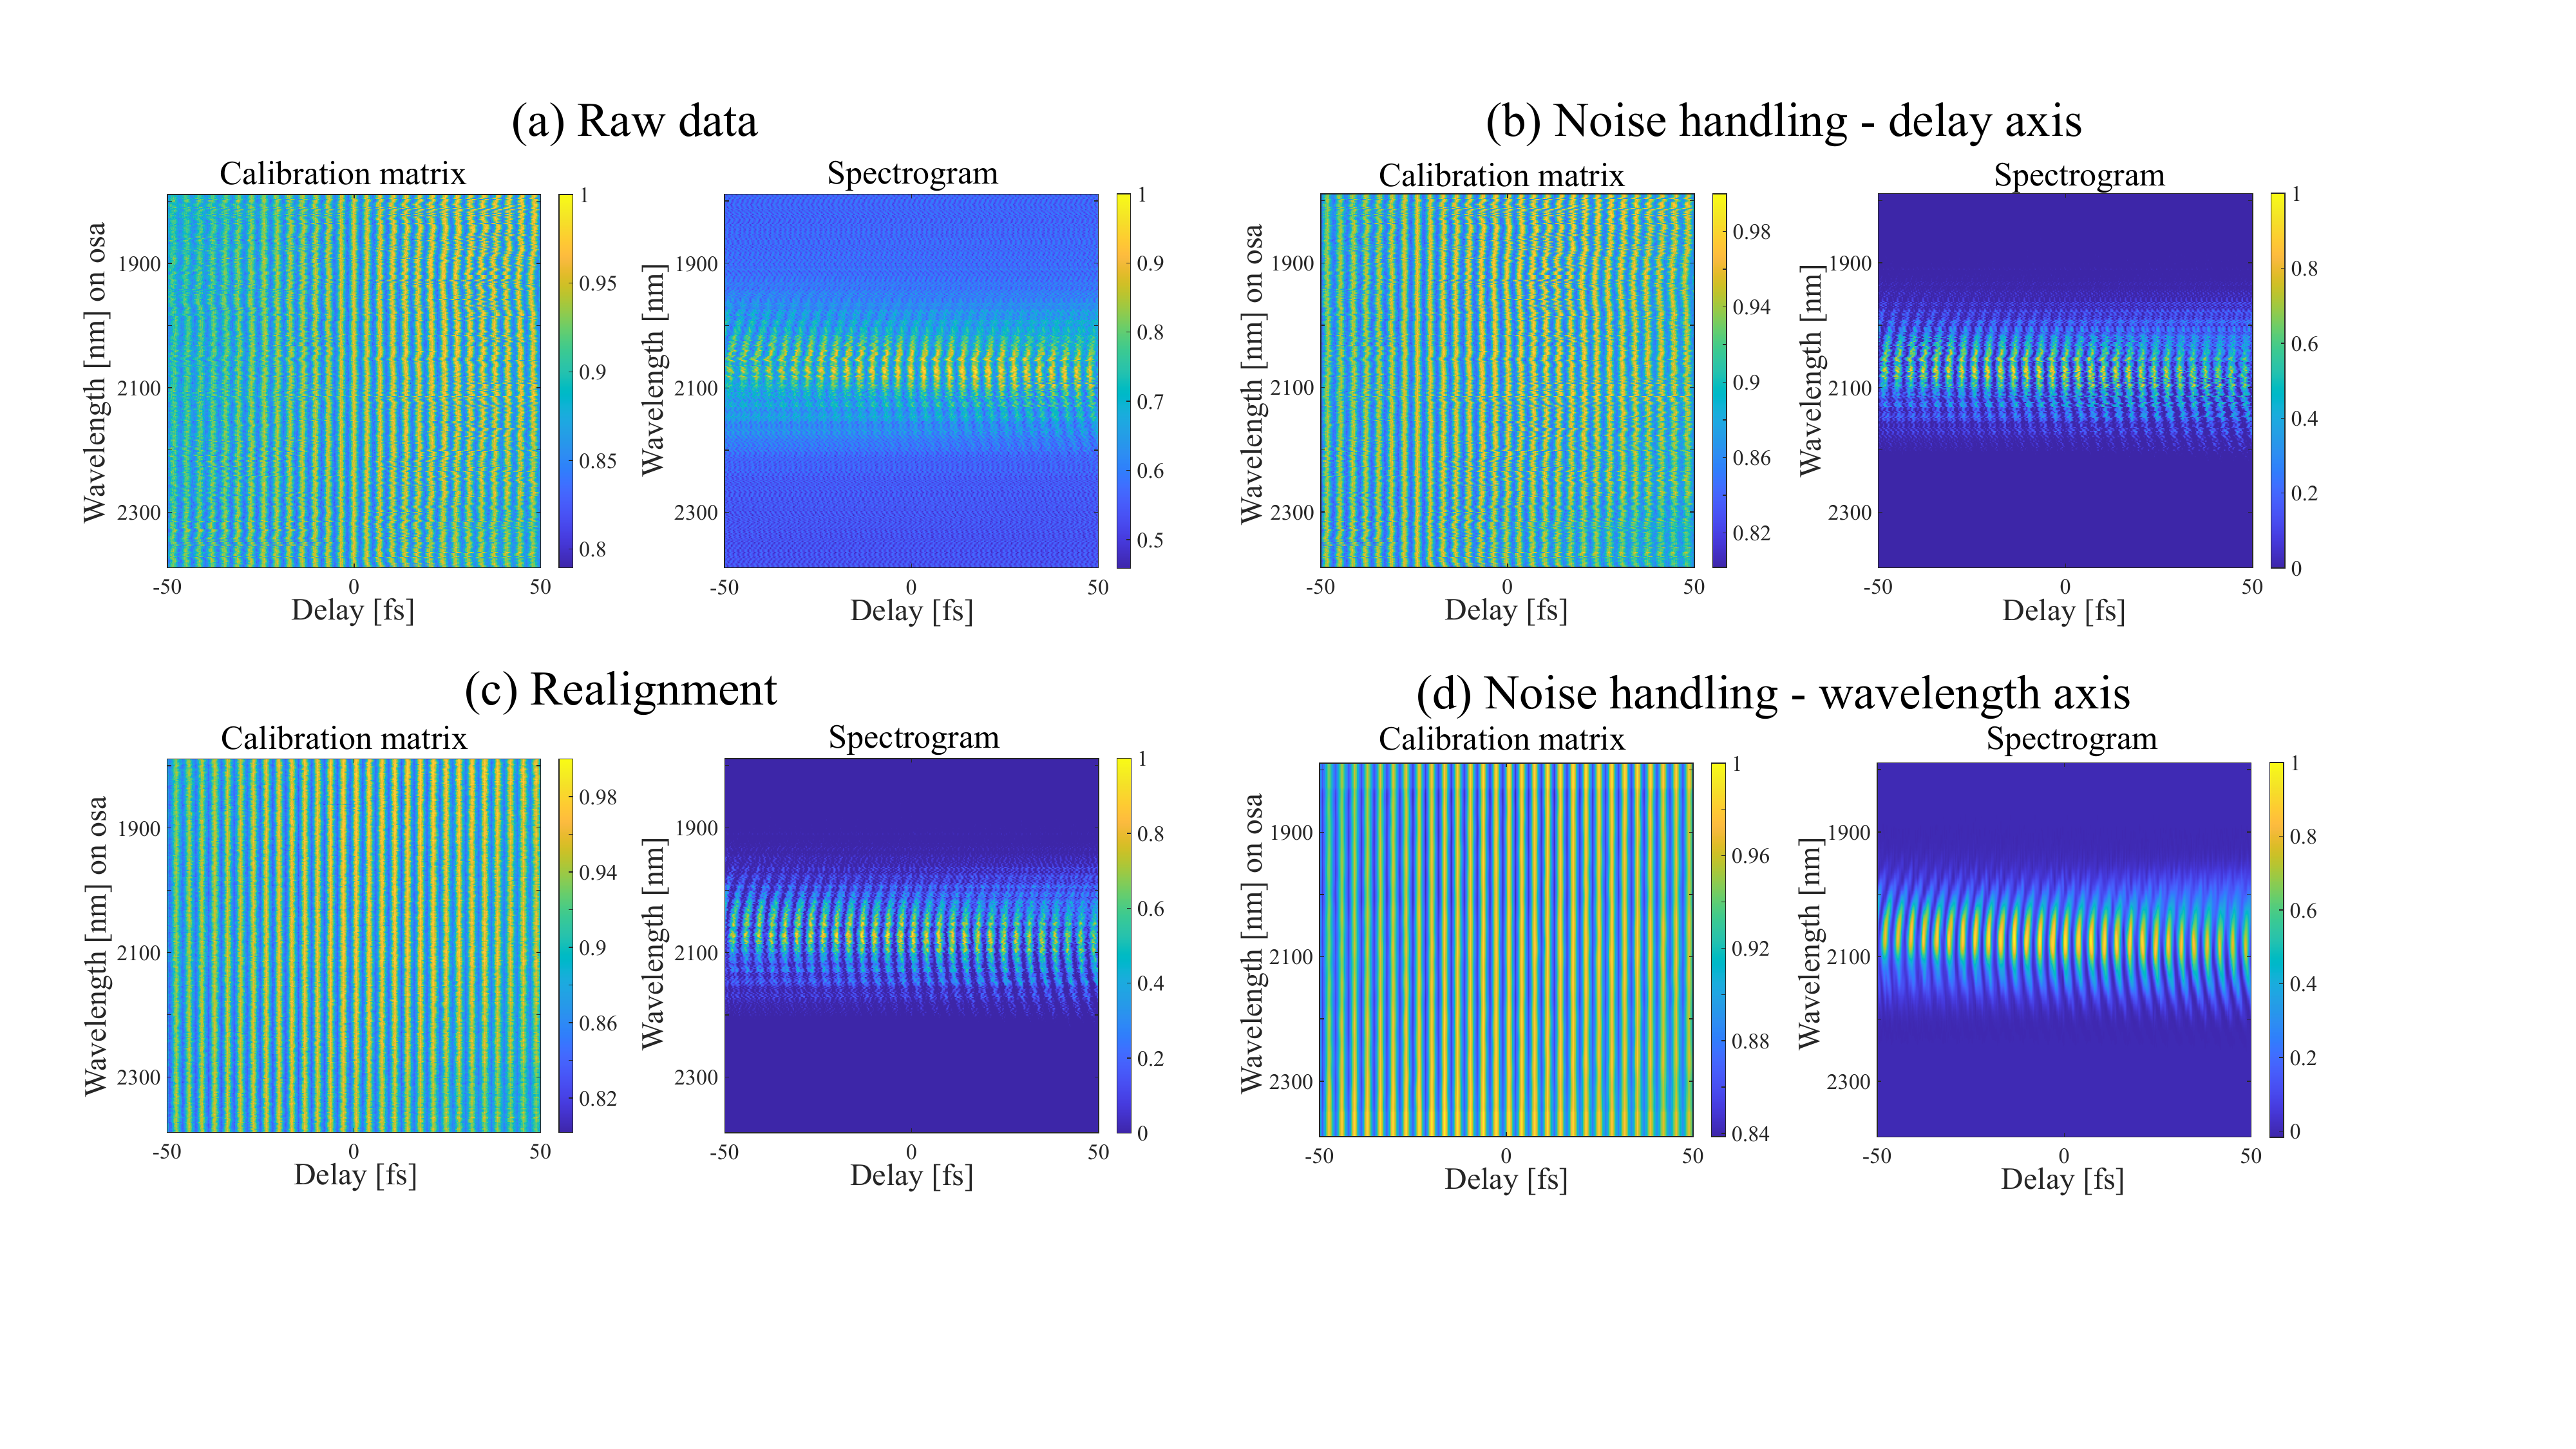}
    % 	}
    	% }
    	\par\end{centering}
        \caption{ \textbf{Postprocessing.} Each sub-panel displays the calibration matrix created from the detector signal and the spectrogram created from the spectrometer signal at each step of the postprocessing.
        (I) displays the raw data collected from the experimental measurement. 
        (II) displays the matrices after lowpass filtering along the
        delay axes for both the matrices and thresholding the spectrogram.
        (III) displays the result of realignment and linearization. 
        (IV) displays the result of lowpass filtering the wavelength axis and renormalization. 
    	}
	\label{fig:sup-postproc}
\end{figure}
The degenerate parametric amplification process is sensitive to the phase difference between the carrier frequencies of the unknown signal and the known gate pulse. 
This results in the nonlinear process being extremely sensitive to experimental variations such as timing jitter between pulses, path length differences caused by thermal fluctuations, alignment variations, stage non-repeatability/non-linearity, etc. 
This phase sensitivity makes it challenging to record a reliable spectrogram using the standard FROG technique due to the slow nature of the measurement. 

To account for these experimental variations, we use a variation of the traditional FROG measurement technique that allows us to generate a calibration signal. 
In a standard FROG, the intensity spectrogram is generated by recording all frequency components simultaneously for each distinct delay value in an iterative manner. 
This would be equivalent to iteratively filling each column in the spectrograms.
Here, we record all the delay values for each distinct frequency component in an iterative manner (in other words, iteratively filling each row in the spectrogram). 
This is done experimentally by scanning the stage and recording the output signal one frequency component at a time. 
Experimentally this was done by sequentially measuring contributions to wavelengths from $1890 nm$ to $2390 nm$ with a bandwidth of $2nm$.  
This allows us to use an additional slow detector that can be used as a calibration tool. 

In an ideal case, the slow detector would be expected to record the same signal from one iteration to the next. 
Any variations in the recorded signal can hence be attributed to experimental fluctuations that can now be calibrated for. 
The calibration process includes noise handling and realignment. 
The noise handling accounts for electronic noise, optical power fluctuations, and is achieved through low-pass filtering, thresholding, and renormalization.
The realignment procedure accounts for optical phase variations that can be caused due to timing jitter between pulses, stage nonrepeatability/nonlinearity, etc. 
The phase variations appear as nonrepeating rows in the calibration matrix.
These variations are calibrated for by compensating for them from one iteration to the next in the calibration matrix and applying the identical changes to the corresponding spectrogram.
This is done in two steps - we first realign the carrier and the envelope of each row of the calibration matrix to the first row. 
We then linearize the calibration matrix by interpolating the peaks and troughs of each row to be the expected distance of $\pi /2$ apart (where $2\pi$ corresponds to one optical cycle at the signal wavelength). 
This $\pi/2$ difference is analytically true only for transformed limited pulses.
However, for dispersed pulses, the distance between an adjacent peak and trough was heuristically found to be close to $\pi/2$ through simulations.
Additionally, the overdetermined \cite{trebino2000frequency} nature of the FROG retrieval algorithm, enables the successful retrieval of chirped pulses even with this transformation. 
Figure \ref{fig:sup-postproc} describes the postprocessing workflow. 
Each panel contains the calibration matrix (detector signal) and the corresponding spectrogram. 
Fig. \ref{fig:sup-postproc} (I) shows a zoomed-in version of the raw data that is collected from the measurement. 
Notice the variations between the different rows of the calibration matrix. 
Fig. \ref{fig:sup-postproc} (II) shows the calibration matrix and spectrogram after low pass filtering the delay axis of both matrices and thresholding the spectrogram. 
The threshold for the spectrogram was set to the maximum value at $1800 nm$ (which determines the spectrometer noise level since no signal is expected).
The calibration matrix and corresponding spectrogram values are then realigned and linearized and are displayed in Fig. \ref{fig:sup-postproc} (III). 
Finally, the matrices are passed through a low pass filter along the frequency axis resulting in Fig. \ref{fig:sup-postproc} (IV).

\section{Gradient descent}
As mentioned in the main text, the OPA process can be mathematically modeled as follows
\begin{equation}
    E^{DOPA}(t, \tau) = E(t)\cosh(\kappa |G(t-\tau)|) + iE^*(t)\sinh(\kappa|G(t-\tau)|)\exp(i\measuredangle G(t-\tau)) 
    \label{Eq: supFieldDOPA}
\end{equation}
where $E^{DOPA}(t, \tau)$ is the pulse emerging from the degenerate amplification process, $E(t)$ is the unknown signal pulse to be measured, $G(t)$ is the gate pulse that pumps the OPA, and $\tau$ is the time delay between the signal and the pump. 
$\kappa = \frac{2zd_{eff}\omega^2}{kc^2}$ is the gain parameter for the OPA where $d_{eff}$ is the nonlinear coefficient, z is the length of the OPA, and $\omega, k$ are the angular frequency and wavenumber of the signal respectively. 

The recovery algorithm follows the standard generalized projects algorithm with a modified loss function to account for the new nonlinearity constraint. 
The loss function, $Z$, can be written as
\begin{equation}
    Z_{DOPA} = \sum_{i,j=1} ^N |E_{DOPA}^{(k)} (t_i, \tau_j) - E_{DOPA}^{(k+1)} (t_i, \tau_j)|^2 
    \label{Eq: supLossFunc}
\end{equation}
where $E_{DOPA}^{(k)} (t_i, \tau_j)$ is the complex interferogram from the $kth$ iteration. 
The goal is to find the electric field $E^{(k+1)} (t)$ that satisfies the nonlinearity condition defined in Eq. \ref{Eq: supFieldDOPA} and minimizes the functional distance $Z_{DOPA}$.

The minimization is performed through gradient descent for which the gradient $-\partial Z/\partial E^{(k+1)} (t_i)$ were calculated analytically for the real and imaginary parts to be 

\begin{equation}
\begin{split}
\frac{ \partial Z_{DOPA}}{\partial Re\{E(t^{(k+1)}_l)\}} = \sum_{j=1} ^N & (-E_{DOPA}^{*(k)} (t_l, \tau_j)f(t_l-\tau_j) - E_{DOPA}^{*(k)} (t_l, \tau_j)g(t_l-\tau_j)) \\
& + E^{*(k+1)} (t_l)|f(t_l-\tau_j)|^2 + E^{*(k+1)} (t_l)f^*(t_l-\tau_j)g(t_l-\tau_j) \\
& + E^{(k+1)} (t_l)g^*(t_l-\tau_j)f(t_l-\tau_j) + E^{(k+1)} (t_l)|g(t_l-\tau_j)|^2) \\
& + c.c.,     \\
\frac{ \partial Z_{DOPA}}{\partial Im\{E(t^{(k+1)}_l)\}} = \sum_{j=1} ^N & (-iE_{DOPA}^{*(k)} (t_l, \tau_j)f(t_l-\tau_j) + iE_{DOPA}^{*(k)} (t_l, \tau_j)g(t_l-\tau_j)) \\
& + iE^{*(k+1)} (t_l)|f(t_l-\tau_j)|^2 - iE^{*(k+1)} (t_l)f^*(t_l-\tau_j)g(t_l-\tau_j) \\
& + iE^{(k+1)} (t_l)g^*(t_l-\tau_j)f(t_l-\tau_j) - iE^{(k+1)} (t_l)|g(t_l-\tau_j)|^2) \\
& + c.c.,    \\
\end{split}
\end{equation}
respectively where $f(t) = \cosh(\kappa |G(t)|)$ and $ g(t) = i\sinh(\kappa|G(t)|)\exp(i\measuredangle G(t))$ have been used as variables for simplification \cite{trebino2000frequency}.
